# Supplementary material for: Learning Preconditioner for Conjugate Gradient PDE Solvers
Source: arXiv:2305.16432 source file (2023-09-06)
Supplement: Supplementary file 2 [file supp-environment-bak.tex]

\begin{table}[htb]
    \centering
    \begin{scriptsize}
    \begin{tabular}{c|c|c|c|c|c}
    \toprule
        PDE &  Mesh Shape & Number of Nodes & Number of Elements & Physics Parameter & Boundary Condition\\ 
    \midrule
        heat-2d & eight shaped mesh& 7454 & 14351 & diffusivity: 10.0 & varying \\
        wave-2d & circle shaped mesh &4852 & 8839 & speed: 0.1 & varying \\
        poisson-2d& cynlinder flow & 3167 & 6117 & density: 0.01 & varying \\
        poisson-3d & connector mesh & 23300 & 129981 & - & fixed \\
        poisson-3d & armadillo mesh & 18181 & 97476 & - & fixed \\
    \bottomrule
    \end{tabular}
    \end{scriptsize}
    \caption{Environment setup for experiment section~\ref{sec:exp:network}, section~\ref{sec:exp:classic},  section~\ref{sec:exp:loss}, section~\ref{sec:exp:generalize},}
    \label{table:environment_table}
\end{table}
